# Supplementary material for: Analog Beamforming Codebooks for Wideband Full-Duplex Millimeter-Wave Systems
Source: arXiv:2411.03691 source file (2024-11-06)
Supplement: Supplementary file 1 [file sec-appendix.tex]

\appendices

\section{Test}
